# Supplementary material for: Keyboards as a new model of computation
Source: arXiv:2102.10182 source file (2021-07-01)
Supplement: Supplementary file 1 [file rek_algebrique_si_besoin.tex]

\subsubsection[]{Preuve du \myref{thm-rek_in_alg}}

\label{proof-rek_in_alg}

\ThmREKAlg*

\begin{Preuve}
Soit $K \s (T,F)$ un clavier de \REK, soit $\Auto{K}$ l'automate à pile non-déterministe tel que :

\begin{itemize}
    \item Son ensemble d'états est $\Pref(T \cup F) \cup \set{\Fin}$.

    \item Son alphabet d'entrée est $A$, son alphabet de pile est $A \cup \set{\bot}$, $\bot$ étant le symbole de fond de pile.

    \item $\epsilon$ est le seul état initial

    \item $\Fin$ est le seul état final. L'automate accepte uniquement dans l'état $\Fin$ avec une pile vide.

    \item L'ensemble des transitions est
    $\Delta = \Delta_A \cup \Delta_{\retour} \cup \Delta_{\text{boucle}} \cup \Delta_{\Fin}$
    avec

\begin{align*}
    \Delta_{A} =
        &\set{t \transpile{\epsilon}{\rien}{\depile a} ta \mid ta \in \Pref(T \cup F), a \in A}\\
    \Delta_{\retour} =
        &\set{t \transpile{\epsilon}{\empile a}{\rien} t\retour \mid t\retour \in \Pref(T \cup F), a \in A} \cup \\
        &\set{t \transpile{\epsilon}{\empile \bot}{\depile \bot} t\retour \mid t\retour \in \Pref(T \cup F)}\\
    \Delta_{\text{boucle}} =
        &\set{t \transpile{\epsilon}{\rien}{\rien} \epsilon \mid t \in T}\\
    \Delta_{\Fin} =
        &\set{t \transpile{\epsilon}{\rien}{\rien} \Fin \mid t \in F} \cup\\
        &\set{\Fin \transpile{a}{\empile a}{\rien} \Fin \mid a \in A} \cup\\
        &\set{\Fin \transpile{ \epsilon}{\empile \bot}{\rien} \Fin}
\end{align*}
\end{itemize}

On observe qu'un mot $w$ est accepté par $\Auto{K}$ si et seulement si il existe une exécution de l'automate menant à l'état $\Fin$ avec $w\bot$ comme contenu de pile, si et seulement si il existe $t \in F$ et $w' \in A^*$ tels qu'il existe une exécution de $\Auto{K}$ menant à $\epsilon$ avec $w'\bot$ comme contenu de pile, et $w' \cdot t =w$.

De plus une induction sur $n$ nous montre que pour toute exécution de $\Auto{K}$ de longueur $n$ menant à un état $p \in \Pref(T)$, il existe un mot $w$ et une suite de touches $t_1 \cdots t_k \in T^*$ tels que $\epsilon \cdot t_1 \cdots t_kp = \miroir{w}$ et le contenu de pile soit $w \bot$ à la fin de l'exécution.

Une autre induction sur $n$ nous montre que pour toute suite de $\sigma_1 \cdots \sigma_n$ d'opérations formant un élément de $T^*p$ avec $p\in \Pref(T)$, il existe une exécution de l'automate menant à l'état $p$ avec comme contenu de pile $\miroir{\epsilon \cdot \sigma_1 \cdots \sigma_n} \bot$.

Ces deux inductions nous montrent en particulier que les mots $w$ tels qu'il existe une exécution de $\Auto{K}$ menant à $\epsilon$ avec $w \bot$ dans la pile sont exactement les miroirs des mots $w$ obtenus en appliquant une suite de touches de $T$ à $\epsilon$.

En conclusion, $\Auto{K}$ reconnaît exactement le miroir de $\langage{K}$. Pour tout automate à pile on peut construire en temps polynomial un automate à pile reconnaissant le langage miroir du sien, on obtient donc le résultat.
\end{Preuve}

Enfin, nous présentons en \myref{fig-exemple-automate-rek} l'automate obtenu à partir
du clavier $\set{\touche{\retour^2 abc}, \touche{\retour^4 bb}}$ en utilisant la construction présentée dans la preuve de ce lemme. 
\[
    \boxed{
        \color{red} \act{a} \qquad
        \color{blue} \act{b} \qquad
        \color{green} \act{c} \qquad
        \color{black} \act{\epsilon}\qquad
        \color{red!10} \blacksquare \color{black} : \text{état final} \qquad
        \color{green!10} \blacksquare  \color{black} : \text{état vert}
    }
\]

\begin{figure}[H]
    \centering
    \tikzset{
        main node/.style={
            %ellipse,
            rectangle,
            %fill=green!6, red!10
            %fill=red!10
            draw,
            minimum size=1cm,
            inner sep=1.5pt
        },
    }
    \begin{tikzpicture}
        \node [main node] (0) {0};

        \node [main node, below = 1cm of 0, fill=green!6] (3)
              {$(2, a, bc, a)$};
        \node [main node, left = 1cm of 3, fill=green!6] (2)
              {$(2, ab, c, ab)$};
        \node [main node, left = 1cm of 2, fill=green!6] (1)
              {$(2, abc, \epsilon, abc)$};
        \node [main node, right = 1cm of 3, fill=green!6] (4)
              {$(4, bb, \epsilon, bb)$};
        \node [main node, right = 1cm of 4, fill=green!6] (5)
              {$(4, b, b, b)$};

        \node [main node, below = 1cm of 3] (8)
              {$(2, a, bc, \epsilon)$};
        \node [main node, below = 1cm of 2] (7)
              {$(2, ab, c, b)$};
        \node [main node, below = 1cm of 1] (6)
              {$(2, abc, \epsilon, bc)$};
        \node [main node, below = 1cm of 4] (9)
              {$(4, bb, \epsilon, b)$};
        \node [main node, below = 1cm of 5] (10)
              {$(4, b, b, \epsilon)$};

        \node [main node, below = 1cm of 6] (11)
              {$(2, abc, \epsilon, c)$};
        \node [main node, below = 1cm of 7] (12)
              {$(2, ab, c, \epsilon)$};
        \node [main node, below = 1cm of 9, fill=red!10] (13)
              {$(4, bb, \epsilon, \epsilon)$};

        \node [main node, below = 1cm of 11, fill=red!10] (14)
              {$(2, abc, \epsilon, \epsilon)$};

        \draw[->,thick, >=latex, ] (0) to[bend right=20] (1);
        \draw[->,thick, >=latex, ] (0) to[bend right=15] (2);
        \draw[->,thick, >=latex, ] (0) to (3);
        \draw[->,thick, >=latex, ] (0) to[bend left=15] (4);
        \draw[->,thick, >=latex, ] (0) to[bend left=20] (5);

        \draw[->,thick, >=latex, red] (1) to (6);
        \draw[->,thick, >=latex, red] (2) to (7);
        \draw[->,thick, >=latex, red] (3) to[bend right=30] (8);
        \draw[->,thick, >=latex, blue] (4) to (9);
        \draw[->,thick, >=latex, blue] (5) to (10);

        \draw[->,thick, >=latex, blue] (6) to (11);
        \draw[->,thick, >=latex, blue] (7) to (12);
        \draw[->,thick, >=latex, blue] (9) to (13);

        \draw[->,thick, >=latex, green] (11) to (14);

        \draw[->,thick, >=latex] (8) to[bend right=30] (3);

        \draw[->,thick, >=latex] (8) to[bend left=15] (2);
        \draw[->,thick, >=latex] (8) to[bend right=15] (4);

        \draw[->,thick, >=latex] (8) .. controls +(-4,-9) and +(1.5,-1) .. (1);
        \draw[->,thick, >=latex] (8) .. controls +(4,-9) and +(-1.1,-1) .. (5);
        \draw[->,thick, >=latex] (0, 1.3) to (0);
    \end{tikzpicture}
    \vspace{-3cm}
    \caption{Automate du clavier $\set{\touche{\retour^2 abc}, \touche{\retour^4 bb}}$}
    \label{fig-exemple-automate-rek}
\end{figure}

\begin{Preuve}
    Considérons $t'$, le suffixe de $t$ commençant par $\hat{a}$ et créons
    $P$ un tableau indicé de $1$ à $\size{t'}$. Le but est d'indiquer
    dans la case $i$ de $P$ la position du curseur par rapport à $\hat{a}$ après l'exécution des $i$ premières
    opérations élémentaires de $t'$ (notre origine est juste à droite du $\hat{a}$). Nous posons alors $P[1] = 0$ et pour $0 \leq i < \size{t}$
    \[
        P[i + 1] = \begin{cases*}
            P[i] + 1 & si $t'_i = a \in A$\\
            P[i] - 1 & si $t'_i \in \set{\gauche, \retour}$
        \end{cases*}
    \]
    Une récurrence immédiate sur $i$ montre que tant que $P[i]$
    ne devient pas négatif, $P[i]$ correspond bien à la position
    du curseur par rapport au $\hat{a}$. Posons alors $k$
    l'entier minimal tel que $P[k + 1] < 0$ ou $-1$ si un tel entier n'existe pas.

    Nous allons montrer que le $\hat{a}$ est effacé si
    et seulement si $P[k] = 0$ et $t'_{k + 1} = \retour$.
    \begin{description}
        \item[$\impliedby$] : si $P[k] = 0$ et $t'_{k + 1} = \retour$,
        alors on est juste à droite du $\hat{a}$
        et on efface la lettre à gauche du curseur ; on
        efface bien le $\hat{a}$.
        \item[$\implies$] : supposons que le $\hat{a}$ est effacé.
        Si $k = -1$, alors tous les éléments de $P$ sont positifs,
        ce qui est impossible (on obtient un $-1$ après avoir effacé
        le $\hat{a}$).

        Donc $k \geq 0$ et par définition de $k$, $P[k] \geq 0$ et
        $P[k + 1] < 0$, d'où $t_{k + 1} \in \set{\gauche, \retour}$.
        Mais si $t_{k + 1} = \gauche$, alors le curseur passe à
        gauche du $a$ sans l'avoir effacé ; le \myref{thm-fondamental_grek}
        permet d'exclure cette possibilité.

        Il ne reste qu'une possibilité, $t_{k + 1} = \retour$.
        On obtient $P[k] = 0$ grâce à la définition de $P$
        (l'écart entre $P[k]$ et $P[k + 1]$ est de $1$,
        $P[k + 1] < 0$ et $P[k] \geq 0$).
    \end{description}
    Et on a l'équivalence.

    De plus, $P$ ne dépend que de la touche $t$ et pas de la configuration
    $\config{u}{v}$ considérée. Ainsi, si $\hat{a}$ appartient à
    $\config{u}{v}$, alors pour tout $u', v'$, $\hat{a}$ appartient à
    $\config{u'}{v'}$.
\end{Preuve}
